# Supplementary material for: Practical Bayesian Optimization of Objectives with Conditioning Variables
Source: arXiv:2002.09996 source file (2020-11-02)
Supplement: Supplementary file 1 [file 3-global-on-conditional.tex]

\section{Global algorithms on conditional problems}
Note that state is determined by the algorithm. 
Global optimization algorithms prioritize sampling state-action pairs
with high reward while conditional algorithms prioritize sampling states with high
density and actions with high reward. Thus, if high reward states coincide with high density states, both algorithm types will behave similarly. The ambulance problem may be an instance of this special edge case
as state density is peaked in the centre of the map where journey times may also be
minimized. We have added this hypothesis to the paper and leave a fuller study of
such subtle edge case test problems to future work. Further, R1 commends the inclusion of EI.

% Hence the anomalous EI result may expose a feature of
% the problem and not a feature of the algorithm.

\begin{figure}
\label{fig:synth}
    \centering
    \includegraphics[width=0.75\textwidth]{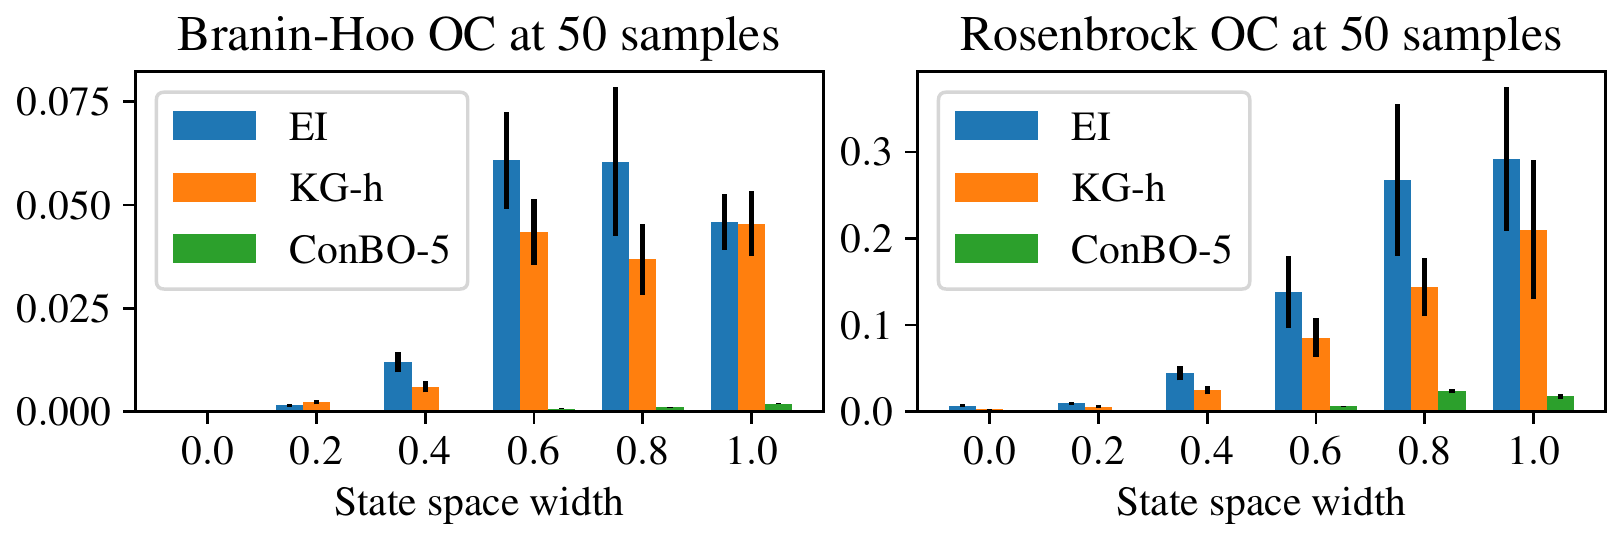}
\end{figure}

To demonstrate the necessity of conditional methods,
we apply EI, hybrid KG and ConBO
to a range of synthetic conditional problems that vary only by the width of the state
space. Zero width means that state space is a single state, the problem
reduces to global optimization and all methods achieve
near zero OC. As width increases to 1 (full state space), there are more states to optimize and
ConBO optimizes each state consistently achieving near zero OC while
EI and KG do not optimize every state and do not converge (see Figure \ref{fig:synth}). We have included this experiment and discussion in the paper.
