# Supplementary material for: Practical Bayesian Optimization of Objectives with Conditioning Variables
Source: arXiv:2002.09996 source file (2020-11-02)
Supplement: Supplementary file 2 [file Compare-REVI-MTS.tex]

\section{Relation to Previous Methods}
\subsection{REVI}

\begin{itemize}
    \item scaling with dimension
    \item discretization fixed with x^n+1
    \item deteministic optimizer, bias
    \item sparsity trick and convolution trick
    \item 
\end{itemize}

At each iteration the REVI algorithm discretizes the states space $S$ with samples from $\P[s]$ and the action
space with uniform random samples over $X$, the cross product of these sets forms a discretization over the full
state-action domain. Hence, for each state the KG by discretization may be used and the average over states
approximates the total benefit of a new sample. While this method is simple to compute, it suffers multiple
drawbacks that restrict its applicability.

Firstly the curse of dimensionality. With increasing state space
and action space the discretization size must grow exponentially. In the REVI algorithm, the discretization
is frozen and kept constant for each iternation, this allows various computations to be precomputed and cached.
However with exponentially increasing discretization, this corresponds to
exponentially increasing memory requirement. Instead of caching, quantities may be computed on demand and discarded
which reduces memory requirement but then requires exponential time to compute quantities over an exponential
number of points in the discretization. In our implementation, we occasionally found that REVI would run out of memory
and experiments would crash and thus we had to reduce discretization size.

Secondly, discretizing the state space and optimizing an average over discrete states is a biased estimate of the 
true benefit across the infinite continuum of states. In the REVI framework, this can only be remedied by increasing
samples size thereby increasing the discretization. If the sample size is too small, The Monte-Carlo estimate
is poor, if the sample size is large, the algorithm complexity grows as described above.

Thirdly, the algorithm is sensitive to hyperparameters. If the state space discretreization is too low, small $n_s$, 
then a sample at $(s,x)\n1$ may have few or no neighboring states over which to measure the benefit. If the action space
discretization is too small, then for each state, Knowledge Gradient by discretization will be very poor estimate of the
benefit of a new point on that state. Again, in the REVI framework, these can only be remedied by increasing
discretization sizes. In general, if the typical distance between points in the discretization is comparable or
longer than the length scales of the GP model, then REVI acquisition function becomes random.
If the interpoint spacing is much larger, computation significantly slows down.

The ConBO framework does not suffer any of these issues. Firstly, the Monte Carlo integration over states is
stochastic with each call to ConBO. By using the Adam optimizer, the peak that is found at the
end of optimizing ConBO$(s,x)$$ is an unbiased estimate of the true average over infinitely many states.

Secondly, ConBO uses importance sampling, the Monte-Carlo states depend upon $(s,x)\n1$ such that only very
relevant states within GP length scales of $(s,x)\n1$ are included in the integration, thereby reducing variance,
improving approximation accuracy and the convergence of the Adam optimizer.

Thirdly, by using the hybrid KG approach, the benefit of a sample on one state can be estimated very accurately
regardless of the dimensionallity of the action space $X$, one may use $n_z=5$ for any dimensional space and
the {\tt Optimizer}$(\cdot)$ uses gradients and convergence does not scale exponentially with .

In summary, both methods use similar motivation, however REVI is biased, sensitive to hyperparameters
either resulting in poor approximations if the hyperparameters are too low or expensive computation
if they are too high. As a result, REVI can be safely applied in low dimensional simple problems, 
however the algorithm performance becomes very unstable for larger problems. 

ConBO, with stochastic integration and stochastic gradient ascent, importance sampling over states, and
hybrid KG over actions does not suffer these problems and therefore performs much mre reliably over
the range of problems considered.
